# Supplementary material for: How Generalizable Is My Behavior Cloning Policy? A Statistical Approach to Trustworthy Performance Evaluation
Source: arXiv:2405.05439 source file (2024-07-18)
Supplement: Supplementary file 1 [file appendix.tex]

\section{Appendix} \label{appendix}
Although one would certainly be justified in using the CP or DKW bounds, our view is that it is worth the small amount of extra effort to use bounds with optimality properties. In practice, the complexity of each of these bounds is typically abstracted away from the user who will often only need to make a simple function call to a relevant software library. Nevertheless, for the interested reader we provide some comparisons between these more popular methods and the methods we use.

\subsection{Binomial CIs}
As mentioned in \cref{sec:related}, the Clopper-Pearson (CP)~\cite{clopper_pearson} method is the most popular method for constructing binomial CIs that hold with a user-specified confidence. In fact, for the problem of computing a lower confidence bound on the probability of success which is deterministic conditioned on the observations, CP is unimprovable~\cite{wang2006smallest}. This is in contrast to the method we use which leverages an auxiliary random variable in the test statistic such that the method results in a UMA interval (the CP interval is not UMA). 

Here we show some analysis comparing the efficiency of the approach we present vs CP. 

Note that there is not a readily available tool for analyzing the MES of the CP interval. One of the advantages of our approach is that it is amenable to analyzing tightness through MES.

\subsection{CDF Bounds}
Also mentioned in \cref{sec:related}, the DKW inequality~\cite{dvoretzky1956,massart1990} is the most common method for placing upper confidence bounds on CDFs. In \cref{fig:cdf_comp} we show the difference between the offset term $\epsilon$ when computed via the DKW inequality and when computed as in \cref{eq: eps}. The difference is always positive, albeit small. This shows that indeed the DKW method is more conservative than is necessary, but that this conservative diminishes quickly as the number of samples increases or the confidence level decreases.

\begin{figure}[h]
    \centering
    \includesvg[width=\linewidth]{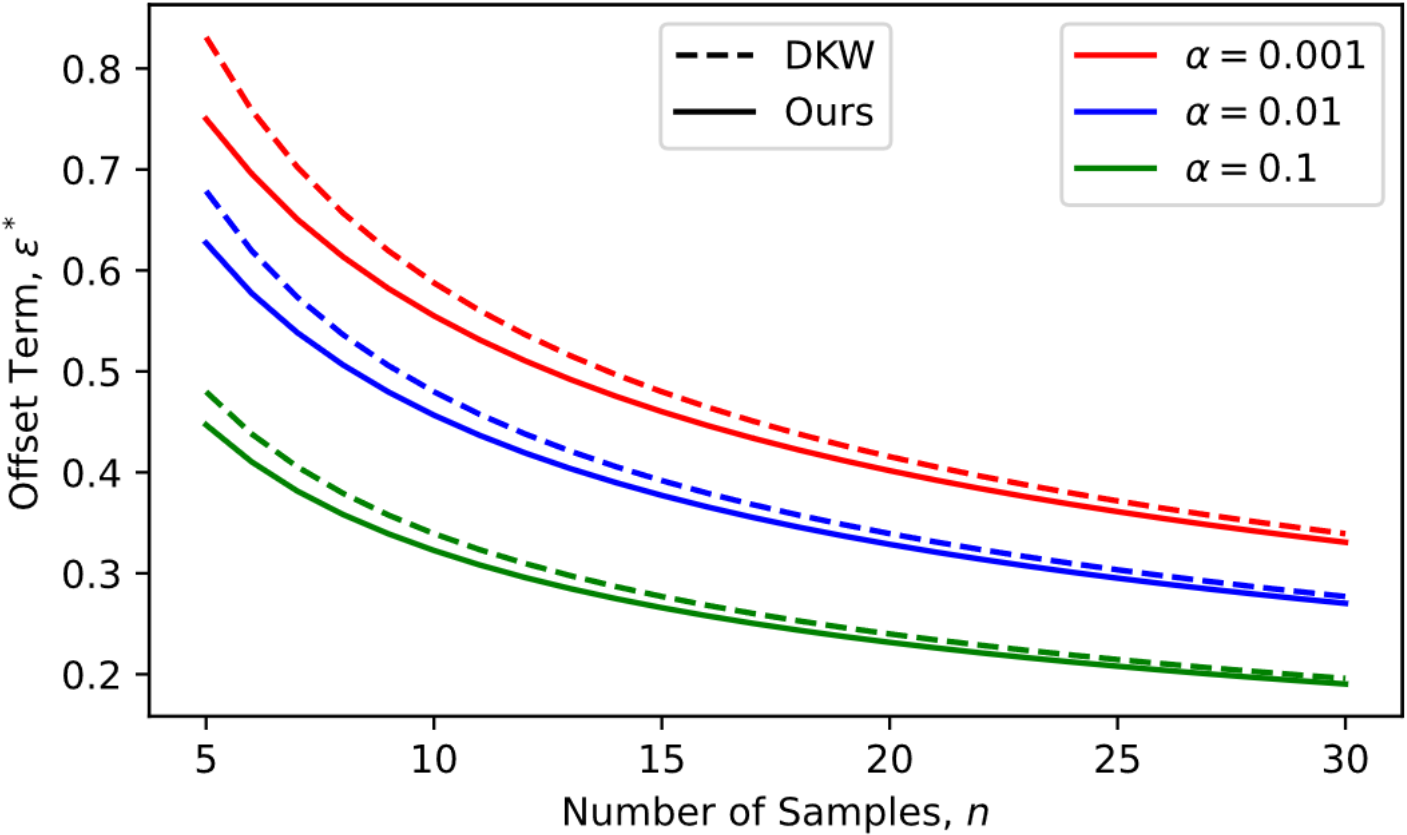}
    \caption{Plotted is the difference between the offset term $\epsilon$ when computed via the DKW inequality and when computed as in \cref{eq: eps} over different sample sizes and different confidence levels.}
    \label{fig:cdf_comp}
\end{figure}

\subsection{Policy Comparison}
In \cref{sec:comparison_ex} we showed how binomial CIs which capture the performance of each policy can be used to also investigate whether one policy performs better than the other. If one is only interested in the relative performance of policies (``policy A has higher success rate than policy B"), then Fisher's and Barnard's tests are the conventional methods for testing this. Note that in practice the relative performance of policies is never the whole story, as one would typically also like to know the absolute performance of each policy as is we provide in our formulation. 

Fisher's and Barnard's tests (see~\cite{two_sample}) are also able to determine (at a $95\%$ confidence level) that the RT-2 policy has higher success rate in each test setting compared to the VC-1 policy. Since Fisher's and Barnard's don't also capture the absolute performance of each policy, they are more efficient in determining the relative performance. More concretely, in \cref{tab:p-values} we compare the p-values reported by each method for testing the hypothesis that the RT-2 policy has a higher success rate than the VC-1 policy against the null hypothesis that the RT-2 policy does not have a higher success rate than the VC-1 policy. Unsurprisingly, Fisher's is more powerful than ours and Barnard's is more powerful than both ours and Fisher's. While the differences in the p-values are quite large, we give more perspective in \cref{tab:sample_sizes} which shows the number of samples each method would need to conclude (at a $95\%$ confidence level) that the RT-2 policy has a higher success rate than the VC-1 policy if the Monte-Carlo success rates from \cref{tab:rt2_comparison} matched the true success rates exactly. In this perspective the trends between methods remain the same, but the gap in efficiency not as extreme as it appeared in \cref{tab:p-values}. It is worth emphasizing once more that Fisher's and Barnard's tests are more efficient because they do not give information about how big the success rate for the RT-2 policy (or VC-1 policy for that matter) is, only that it is bigger than that of the VC-1 policy.

\floatsetup[table]{objectset=centering,capposition=bottom}
\begin{table}[h]
    \begin{tabular}{lccc}  
        & \shortstack{Symbol\\ Understanding} & \shortstack{Reasoning\\ ~} & \shortstack{Human\\ Recognition} \\ \midrule
        Ours   & \num{1E-3} & \num{1E-3} & \num{3E-2} \\
        Fisher's   & \num{2E-12} & \num{6E-10} & \num{1E-3} \\
        Barnard's   & \num{6E-13} & \num{6E-10} & \num{5E-4}
    \end{tabular}
    \caption{Table of p-values for testing whether the RT-2 policy has a higher success rate than the VC-1 policy based off of the results in \cref{tab:rt2_comparison}.}
    \label{tab:p-values}
\end{table}

\floatsetup[table]{objectset=centering,capposition=bottom}
\begin{table}[h]
    \begin{tabular}{lccc}  
        & \shortstack{Symbol\\ Understanding} & \shortstack{Reasoning\\ ~} & \shortstack{Human\\ Recognition} \\ \midrule
        Ours   & $10$ & $25$ & $27$ \\
        Fisher's   & $5$ & $13$ & $12$ \\
        Barnard's   & $4$ & $11$ & $6$
    \end{tabular}
    \caption{Table of sample sizes needed to conclude (at a $95\%$ confidence level) that the RT-2 policy has a higher success rate than the VC-1 policy if the Monte-Carlo success rates in \cref{tab:rt2_comparison} matched the true success rates exactly.}
    \label{tab:sample_sizes}
\end{table}
